# Supplementary material for: Transcoding compositionally: using attention to find more generalizable solutions
Source: arXiv:1906.01234 source file (2019-06-06)
Supplement: Supplementary file 1 [file appendix.tex]

\appendix

\section{Exception learning for SCAN}

\begin{figure}[!h]
\centering

\begin{subfigure}{0.44\textwidth}
\input{Figures/corruption-scan-baseline/corruption-scan-baseline-4.tex}
\caption{Baseline, 4}
\end{subfigure}
\begin{subfigure}{0.44\textwidth}
\input{Figures/corruption-scan-seq2attn/corruption-scan-seq2attn-4.tex}
\caption{Seq2attn, 4}
\end{subfigure}

\begin{subfigure}{0.44\textwidth}
\input{Figures/corruption-scan-baseline/corruption-scan-baseline-32.tex}
\caption{Baseline, 32}
\end{subfigure}
\begin{subfigure}{0.44\textwidth}
\input{Figures/corruption-scan-seq2attn/corruption-scan-seq2attn-32.tex}
\caption{Seq2attn, 32}
\end{subfigure}

\begin{subfigure}{0.44\textwidth}
\input{Figures/corruption-scan-baseline/corruption-scan-baseline-256.tex}
\caption{Baseline, 256}
\end{subfigure}
\begin{subfigure}{0.44\textwidth}
\input{Figures/corruption-scan-seq2attn/corruption-scan-seq2attn-256.tex}
\caption{Seq2attn, 256}
\end{subfigure}

\begin{subfigure}{0.44\textwidth}
\input{Figures/corruption-scan-baseline/corruption-scan-baseline-1024.tex}
\caption{Baseline, 1024}
\end{subfigure}
\begin{subfigure}{0.44\textwidth}
\input{Figures/corruption-scan-seq2attn/corruption-scan-seq2attn-1024.tex}
\caption{Seq2attn, 1024}
\end{subfigure}
\caption{The normalized percentages of exception and target accuracies over time, for the exception learning experiment of the SCAN task.}
\label{fig:corruption-lookup}
\end{figure}

\kris{Include training details (batch size, etc.)?}
